# Supplementary material for: Mixed-valence compounds as polarizing agents for Overhauser dynamic nuclear polarization in solids
Source: arXiv:2103.00997 source file (2021-03-01)
Supplement: Supplementary file 1 [file SuppInfo.pdf]

# Mixed-valence compounds as polarizing agents for Overhauser dynamic nuclear polarization in solids

Andrei Gurinov,<sup>†</sup> Benedikt Sieland,<sup>‡</sup> Andrei Kuzhelev,<sup>¶</sup> Hossam Elgabarty,<sup>§</sup> Thomas D. Kühne,<sup>§</sup> Thomas Prisner,<sup>¶</sup> Jan Paradies,<sup>‡</sup> Marc Baldus,<sup>†</sup> Konstantin L. Ivanov,<sup>||</sup> and Svetlana Pylaeva<sup>\*,§</sup>

<sup>†</sup>NMR Spectroscopy group, Bijvoet Center for Biomolecular Research, Utrecht University, Padualaan 8, 3584, CH Utrecht, The Netherlands

<sup>‡</sup>Department of Chemistry, Paderborn University, Warburger Str. 100, Paderborn, D-33098 Germany

<sup>¶</sup>Goethe University Frankfurt am Main, Institute of Physical and Theoretical Chemistry, Center for Biomolecular Magnetic Resonance, Max von Laue Str. 7, 60438 Frankfurt am Main, Germany

<sup>§</sup>Dynamics of Condensed Matter and Center for Sustainable Systems Design, Chair of Theoretical Chemistry, University of Paderborn, Warburger Str. 100, Paderborn, D-33098 Germany

<sup>||</sup> International Tomography Center, Siberian Branch of the Russian Academy of Sciences, Novosibirsk, 630090, Russia and Novosibirsk State University, Novosibirsk, 630090, Russia

E-mail: svetlana.pylaeva@upb.de

## 1. Synthesis

### 1.1. Synthesis of N<sup>1</sup>,N<sup>1</sup>,N<sup>4</sup>,N<sup>4</sup>-tetrakis(4-methoxyphenyl)benzene-1,4-diamine<sup>1</sup>

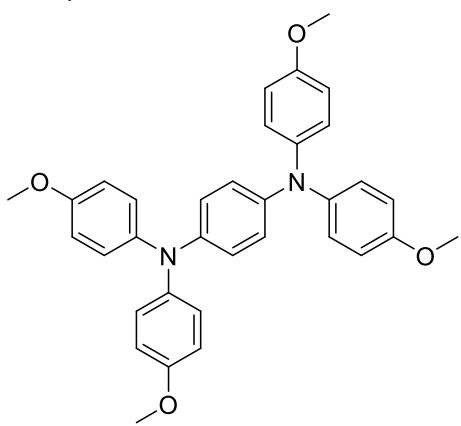

The synthesis was performed analogous to the synthesis of triarylated amines. A 10 mL crimp vial with magnetic stir bar was charged with 4-iodoanisole (257.4 mg, 1.10 mmol, 4.4 eq.), tris(dibenzylideneacetone)dipalladium(0) (8.3 mg, 0.01 mmol, 0.04 eq.), XPhos (26.0 mg, 0.06 mmol, 0.22 eq.), sodium *tert*-butoxide (147.7 mg, 1.54 mmol, 6.16 eq.) and 1,4-diaminobenzene (27.0 mg, 0.25 mmol, 1.0 eq.) and 1,4-dioxane (1.65 mL). The mixture was stirred for 5 h at 110°C, then cooled to RT and quenched with EtOAc

(4 mL). After filtration over Celite, the solvent was removed under reduced pressure. Column chromatography (silica, gradient CH/EE 10:1 to 5:1,  $R_f(5:1)=0.49$ ) and precipitation three times from MeOH (100 mL) gave a nearly colourless, amorphous solid (722.6 mg, 68 %).

**<sup>1</sup>H-NMR** (500 MHz, C<sub>6</sub>D<sub>6</sub>, 303 K,  $\delta$  [ppm]): 7.15-7.11 (m, 8H, CH<sub>Ar</sub>), 7.07 (br., 4H, CH<sub>Ar</sub>), 6.76-6.69 (m, 8H, CH<sub>Ar</sub>), 3.31 (s, 12H, CH<sub>3</sub>).

**<sup>13</sup>C-NMR** (176 MHz, C<sub>6</sub>D<sub>6</sub>, 303 K,  $\delta$  [ppm]): 156.4 (4C, C<sub>q</sub>), 143.9 (2C, C<sub>q</sub>), 142.6 (4C, C<sub>q</sub>), 126.4 (8C, CH<sub>Ar</sub>), 124.2 (4C, CH<sub>Ar</sub>), 115.5 (8C, CH<sub>Ar</sub>), 55.4 (4C, CH<sub>3</sub>).

**<sup>15</sup>N-NMR** (71 MHz, C<sub>6</sub>D<sub>6</sub>; 303 K,  $\delta$  [ppm]): 91.4.

**Mass** (ESI; [m/z]): calculated [M<sup>+</sup>] 532.2362, found [M<sup>+</sup>] 532.2368.

## 1.2. Synthesis of N<sup>1</sup>,N<sup>1</sup>,N<sup>3</sup>,N<sup>3</sup> -tetrakis(4-methoxyphenyl)benzene-1,3-diamine<sup>1</sup>

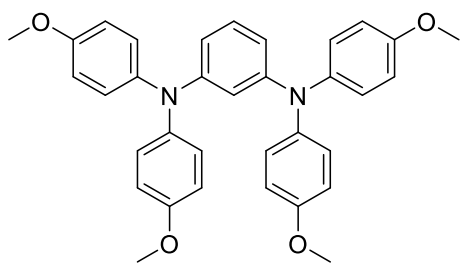

The synthesis was performed analogous to the synthesis of triarylated amines. A 10 mL crimp vial with magnetic stir bar was charged with 4-iodoanisole (257.4 mg, 1.10 mmol, 4.4 eq.), tris(dibenzylideneacetone)dipalladium(0) (8.3 mg, 0.01 mmol, 0.04 eq.), XPhos (26.0 mg, 0.06 mmol, 0.22 eq.), sodium *tert*-

butoxide (147.7 mg, 1.54 mmol, 6.16 eq.), 1,3-diamino benzene (27.0 mg, 0.25 mmol, 1.0 eq.) and 1,4-dioxane (1.65 mL). The mixture was stirred for 5 h at 110°C, then cooled to RT and quenched with EtOAc (4 mL). After filtration over Celite the solvent was removed under reduced pressure. Column chromatography (silica, gradient CH/EE 10:1 to 5:1, R<sub>f</sub>(10:1)=0.19) and precipitation three times from MeOH (100 mL) at -20 °C gave a nearly colourless, amorphous solid (391,0 mg; 37 %).

**<sup>1</sup>H-NMR** (300 MHz, C<sub>6</sub>D<sub>6</sub>, 303 K, δ [ppm]): 7.13-7.07 (m, 8H, CH<sub>Ar</sub>), 7.04 (t, <sup>4</sup>J<sub>HH</sub>=2.2 Hz, 4H, CH<sub>Ar</sub>), 7.02 (t, <sup>3</sup>J<sub>HH</sub>=8.1 Hz, 1H, CH<sub>Ar</sub>), 6.73 (dd, <sup>3</sup>J<sub>HH</sub>=8.1 Hz, <sup>4</sup>J<sub>HH</sub>=2.3 Hz, 2H, CH<sub>Ar</sub>), 6.70-6.64 (m, 8H, CH<sub>Ar</sub>), 3.29 (s, 12H, CH<sub>3</sub>).

**<sup>13</sup>C-NMR** (176 MHz, C<sub>6</sub>D<sub>6</sub>, 303 K, δ [ppm]): 156.6 (4C, C<sub>q</sub>), 150.5 (2C, C<sub>q</sub>), 142.0 (4C, C<sub>q</sub>), 130.3 (1C, CH<sub>Ar</sub>), 127.0 (8C, CH<sub>Ar</sub>), 115.4 (9C, CH<sub>Ar</sub>), 114.8 (2C, CH<sub>Ar</sub>), 55.3 (4C, CH<sub>3</sub>).

**<sup>15</sup>N-NMR** (71 MHz, C<sub>6</sub>D<sub>6</sub>, 303 K, δ [ppm]): 94.5.

**Mass** (ESI, [m/z]): calculated [M<sup>+</sup>] 532.2362, found [M<sup>+</sup>] 532.2363.

## 2. Sample preparation

For DNP measurements, the corresponding closed shell molecule (15 μmol, 1 eq.) was dissolved in 1,1,2,2-tetrachloroethane (1.0 mL, 90D:10H) and the solution was added to the oxidizing agent (15 μmol, 2.6 mg, 1 eq.). The mixture was vigorously shaken and a sample was immediately taken for measurement. This yielded a 15 μM concentration of the radical in the sample.

| Substance                                                                                                    | CAS-number | molecular weight [g/mol] | amount of substance [mmol] | mass [mg] | volume [mL] |
|--------------------------------------------------------------------------------------------------------------|------------|--------------------------|----------------------------|-----------|-------------|
| N <sup>1</sup> ,N <sup>1</sup> ,N <sup>3</sup> ,N <sup>3</sup> -Tetrakis(4-methoxyphenyl)benzene-1,3-diamine | No CAS-No. | 532.64                   | 0.015                      | 8.0       |             |
| N <sup>1</sup> ,N <sup>1</sup> ,N <sup>4</sup> ,N <sup>4</sup> -Tetrakis(4-methoxyphenyl)benzene-1,4-diamine | No CAS-No. | 532.64                   | 0.015                      | 8.0       |             |
| Nitrosyl hexafluorophosphate                                                                                 | 16921-91-8 | 174.97                   | 0.015                      | 2.6       |             |
| 1,1,2,2-Tetrachlorethane-d2                                                                                  | 33685-54-0 |                          |                            |           | 0.9         |
| 1,1,2,2-Tetrachlorethane                                                                                     |            |                          |                            |           | 0.1         |
| α,γ-Bisdiphenylene-β-phenylallyl                                                                             | 35585-94-5 | 495.63                   | 0.02                       | 7.4       |             |

For EPR measurements, the corresponding closed shell molecule (15 μmol, 1 eq.) was dissolved in 1,1,2,2-tetrachloroethane (1.0 mL); and the solution was added to the oxidizing agent (15 μmol, 2.6 mg, 1 eq.). The mixture was vigorously shaken. 0.1 ml of the mixture was taken out of the solution and dissolved in 0.9 ml of 1,1,2,2-tetrachloroethane. A sample was immediately taken for measurement. This yielded a 1.5 μM concentration of the radical in the sample.

| Substance | CAS-number | molecular weight [g/mol] | amount of substance [mmol] | mass [mg] | volume [mL] |
|-----------|------------|--------------------------|----------------------------|-----------|-------------|
|-----------|------------|--------------------------|----------------------------|-----------|-------------|



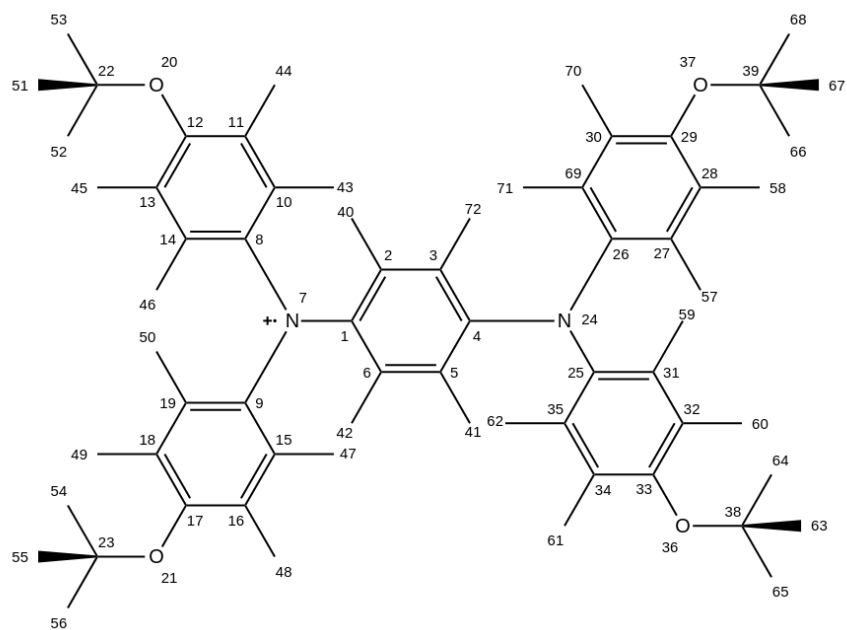

| Atom     | MHz       | Atom     | MHz       | Atom     | MHz      | Atom     | MHz      |
|----------|-----------|----------|-----------|----------|----------|----------|----------|
| 1 C(13)  | -2.22777  | 19 C(13) | 10.11654  | 37 O(17) | -2.72128 | 55 H(1)  | 1.30580  |
| 2 C(13)  | 0.80459   | 20 O(17) | -2.72136  | 38 C(13) | -0.61766 | 56 H(1)  | 1.71791  |
| 3 C(13)  | 0.80461   | 21 O(17) | -2.72137  | 39 C(13) | -0.61766 | 57 H(1)  | -2.78046 |
| 4 C(13)  | -2.22772  | 22 C(13) | -0.61769  | 40 H(1)  | -2.13757 | 58 H(1)  | 1.26688  |
| 5 C(13)  | 0.80460   | 23 C(13) | -0.61769  | 41 H(1)  | -2.13757 | 59 H(1)  | -2.78046 |
| 6 C(13)  | 0.80460   | 24 N(14) | 18.10063  | 42 H(1)  | -2.13757 | 60 H(1)  | 1.26688  |
| 7 N(14)  | 18.10085  | 25 C(13) | -16.77101 | 43 H(1)  | -2.78054 | 61 H(1)  | 1.90847  |
| 8 C(13)  | -16.77127 | 26 C(13) | -16.77102 | 44 H(1)  | 1.26690  | 62 H(1)  | -3.30635 |
| 9 C(13)  | -16.77128 | 27 C(13) | 8.93835   | 45 H(1)  | 1.90851  | 63 H(1)  | -0.06781 |
| 10 C(13) | 8.93840   | 28 C(13) | -4.65712  | 46 H(1)  | -3.30648 | 64 H(1)  | 1.71795  |
| 11 C(13) | -4.65737  | 29 C(13) | 6.09124   | 47 H(1)  | -2.78055 | 65 H(1)  | 1.30567  |
| 12 C(13) | 6.09145   | 30 C(13) | -6.14693  | 48 H(1)  | 1.26690  | 66 H(1)  | -0.06781 |
| 13 C(13) | -6.14719  | 31 C(13) | 8.93835   | 49 H(1)  | 1.90851  | 67 H(1)  | 1.71797  |
| 14 C(13) | 10.11652  | 32 C(13) | -4.65712  | 50 H(1)  | -3.30648 | 68 H(1)  | 1.30566  |
| 15 C(13) | 8.93841   | 33 C(13) | 6.09122   | 51 H(1)  | -0.06786 | 69 C(13) | 10.11641 |
| 16 C(13) | -4.65738  | 34 C(13) | -6.14692  | 52 H(1)  | 1.30581  | 70 H(1)  | 1.90847  |
| 17 C(13) | 6.09146   | 35 C(13) | 10.11642  | 53 H(1)  | 1.71788  | 71 H(1)  | -3.30634 |
| 18 C(13) | -6.14719  | 36 O(17) | -2.72127  | 54 H(1)  | -0.06785 | 72 H(1)  | -2.13757 |

**CASSCF(3,3)/def2-TZVP results:** Loewdin spin densities

|                                                                                    |                |               |               |
|------------------------------------------------------------------------------------|----------------|---------------|---------------|
| 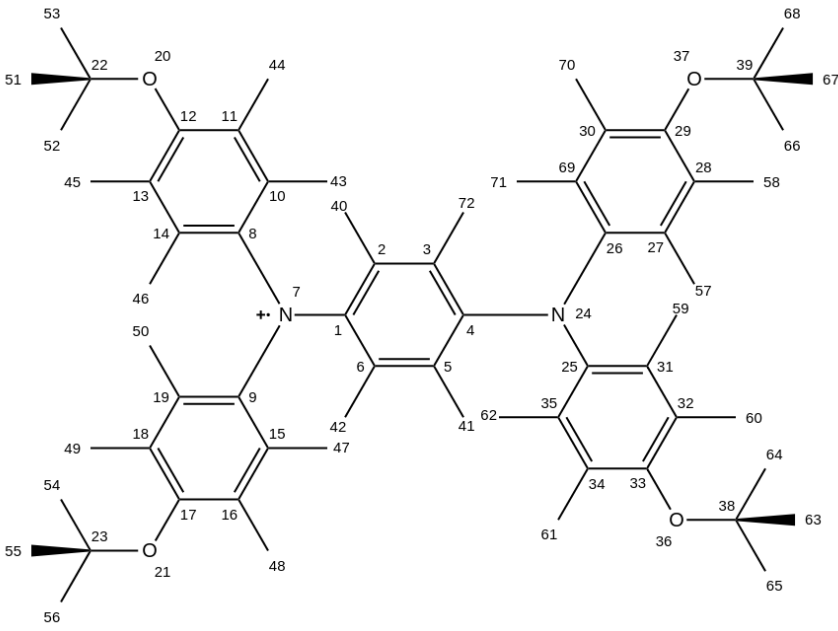 |                |               |               |
| 1 C 0.081212                                                                       | 19 C 0.035023  | 37 O 0.000539 | 55 H 0.000245 |
| 2 C 0.034608                                                                       | 20 O 0.007350  | 38 C 0.000066 | 56 H 0.000268 |
| 3 C 0.010948                                                                       | 21 O 0.007196  | 39 C 0.000079 | 57 H 0.000005 |
| 4 C 0.029455                                                                       | 22 C 0.001105  | 40 H 0.000651 | 58 H 0.000001 |
| 5 C 0.014506                                                                       | 23 C 0.001082  | 41 H 0.000339 | 59 H 0.000023 |
| 6 C 0.035018                                                                       | 24 N 0.015281  | 42 H 0.000650 | 60 H 0.000031 |
| 7 N 0.365500                                                                       | 25 C 0.003234  | 43 H 0.000661 | 61 H 0.000040 |
| 8 C 0.068956                                                                       | 26 C 0.001726  | 44 H 0.000198 | 62 H 0.000132 |
| 9 C 0.068516                                                                       | 27 C 0.000326  | 45 H 0.000211 | 63 H 0.000000 |
| 10 C 0.032065                                                                      | 28 C 0.000220  | 46 H 0.000819 | 64 H 0.000018 |
| 11 C 0.011452                                                                      | 29 C 0.003042  | 47 H 0.000640 | 65 H 0.000017 |
| 12 C 0.026451                                                                      | 30 C 0.003173  | 48 H 0.000199 | 66 H 0.000000 |
| 13 C 0.011756                                                                      | 31 C 0.001548  | 49 H 0.000211 | 67 H 0.000019 |
| 14 C 0.035657                                                                      | 32 C 0.001498  | 50 H 0.000801 | 68 H 0.000018 |
| 15 C 0.031541                                                                      | 33 C 0.001696  | 51 H 0.000000 | 69 C 0.001430 |
| 16 C 0.011302                                                                      | 34 C 0.001624  | 52 H 0.000248 | 70 H 0.000060 |
| 17 C 0.025903                                                                      | 35 C -0.001168 | 53 H 0.000275 | 71 H 0.000172 |
| 18 C 0.011471                                                                      | 36 O 0.000392  | 54 H 0.000001 | 72 H 0.000266 |

#### 4. EPR results

The g- tensors of all studied radicals were obtained from simulation of G-band EPR spectra with EasySpin program<sup>2</sup> using function pepper, corresponding to the solid-state regime. Obtained g-tensor are listed in table.

| Radical   | Solvent | Line width at 10% intensity | g tensor |
|-----------|---------|-----------------------------|----------|
| BDPA      | TCE     | 70 MHz                      | 2.00292  |
|           |         |                             | 2.00269  |
|           |         |                             | 2.00238  |
| 1-4-amine | TCE     | 130 MHz                     | 2.00359  |
|           |         |                             | 2.00309  |

|                  |     |         |         |
|------------------|-----|---------|---------|
|                  |     |         | 2.00288 |
| <b>1-3-amine</b> | TCE | 115 MHz | 2.00349 |
|                  |     |         | 2.00296 |
|                  |     |         | 2.00283 |
|                  |     |         |         |

Table S1. Simulated g-tensors for the set of studied radicals.

**Spectroscopic properties of studied radicals at 295 K in TCE:** the isotropic hyperfine constants ( $a_{\text{iso}}$ , n - number of equivalent nuclei) and peak-to-peak line widths (LW). The X-band EPR spectra were simulated with EasySpin program<sup>2</sup> using function garlic.

| Radical   | $g_{\text{iso}}$ | $a_{\text{iso}}$ / MHz |                     | LW / mT  |            |
|-----------|------------------|------------------------|---------------------|----------|------------|
|           |                  | $^1\text{H}$ (n)       | $^{14}\text{N}$ (n) | Gaussian | Lorentzian |
| BDPA      | 2.002663         | 5.20 (4) 5.57 (4)      | -                   | 0.1102   | 0.1138     |
| 1-4-amine | 2.003186         |                        | 16.00 (2)           | 0.3480   | 0.1024     |
| 1-3-amine | 2.003093         | 4.78 (2)               | 9.09 (2)            | 0.2106   | 0.2325     |

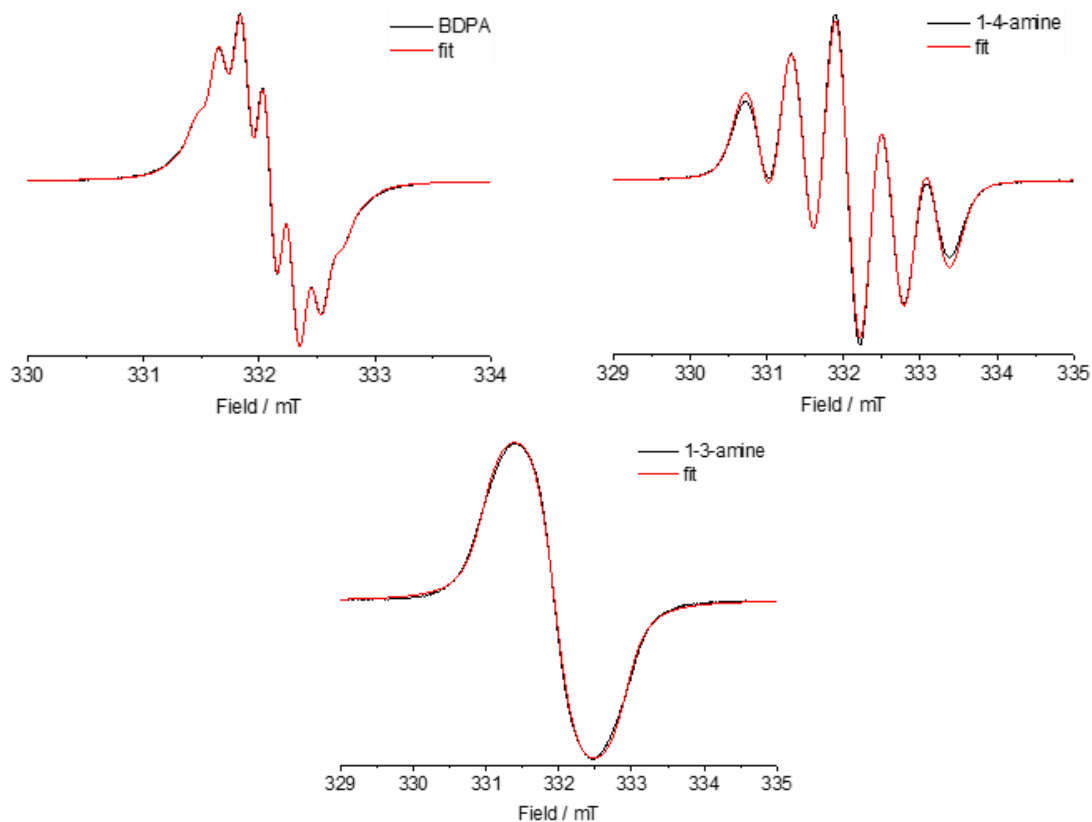

Figure S1. CW EPR spectra of radicals in TCE at room temperature.

## 5. DNP results

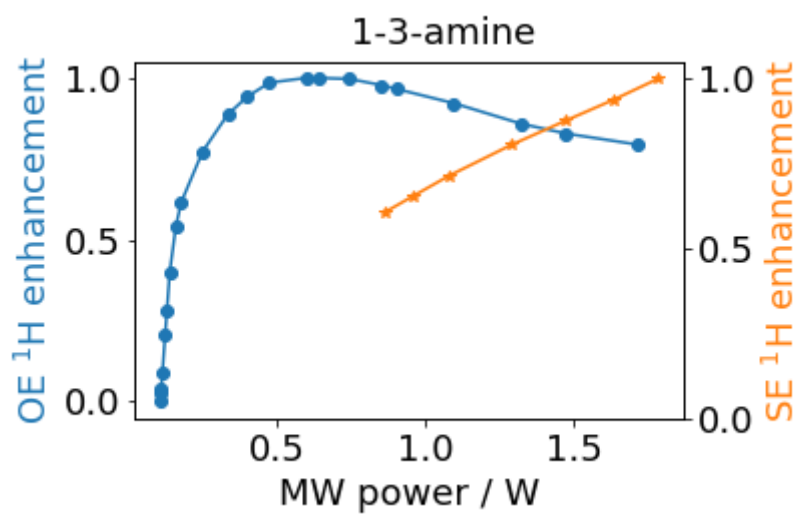

Figure S2. Enhancement as a function of MW power for different components of the field profile for 1-3-amine radical.

## 6. Literature

- (1) Surry, D. S.; Buchwald, S. L. *J. Am. Chem. Soc.* **2007**, *129* (34), 10354–10355.
- (2) Stoll, S.; Schweiger, A. *J. Magn. Res.* **2006**, *178*, 42 – 55
